# Supplementary material for: Nanostructured LaFeO$_{3}$-MoS$_{2}$ for efficient photodegradation and photocatalytic hydrogen evolution
Source: arXiv:2111.03139 source file (2021-11-04)
Supplement: Supplementary file 1 [file appendix1.tex]

\section{Supplementary Material} \label{sec:appendix}
    Here the ESI will be included.
